# Supplementary material for: Collective sleep and activity patterns of college students from wearable devices
Source: arXiv:2412.17969 ancillary file (2024-12-23)
Supplement: Supplementary file 1 [file supp.pdf]

## Supplementary Information: *Collective sleep and activity patterns of college students from wearable devices*

### S-I. FIGURES: COMPLIANCE

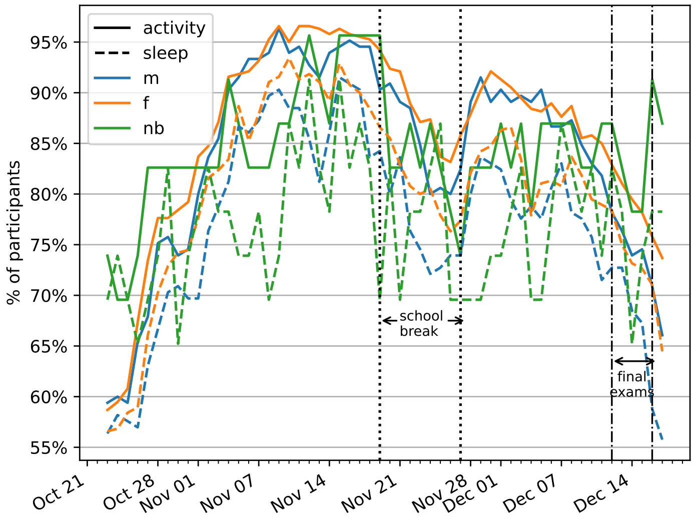


Figure S1. **Ring wear compliance of users by gender.**

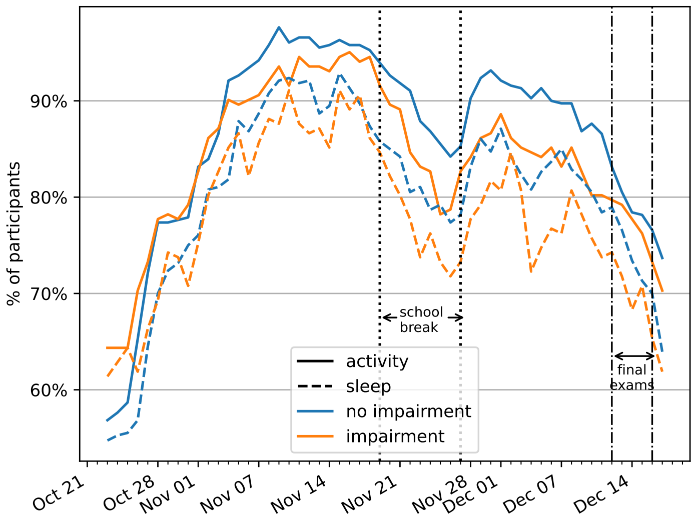


Figure S2. **Ring wear compliance of users by impairment status.**

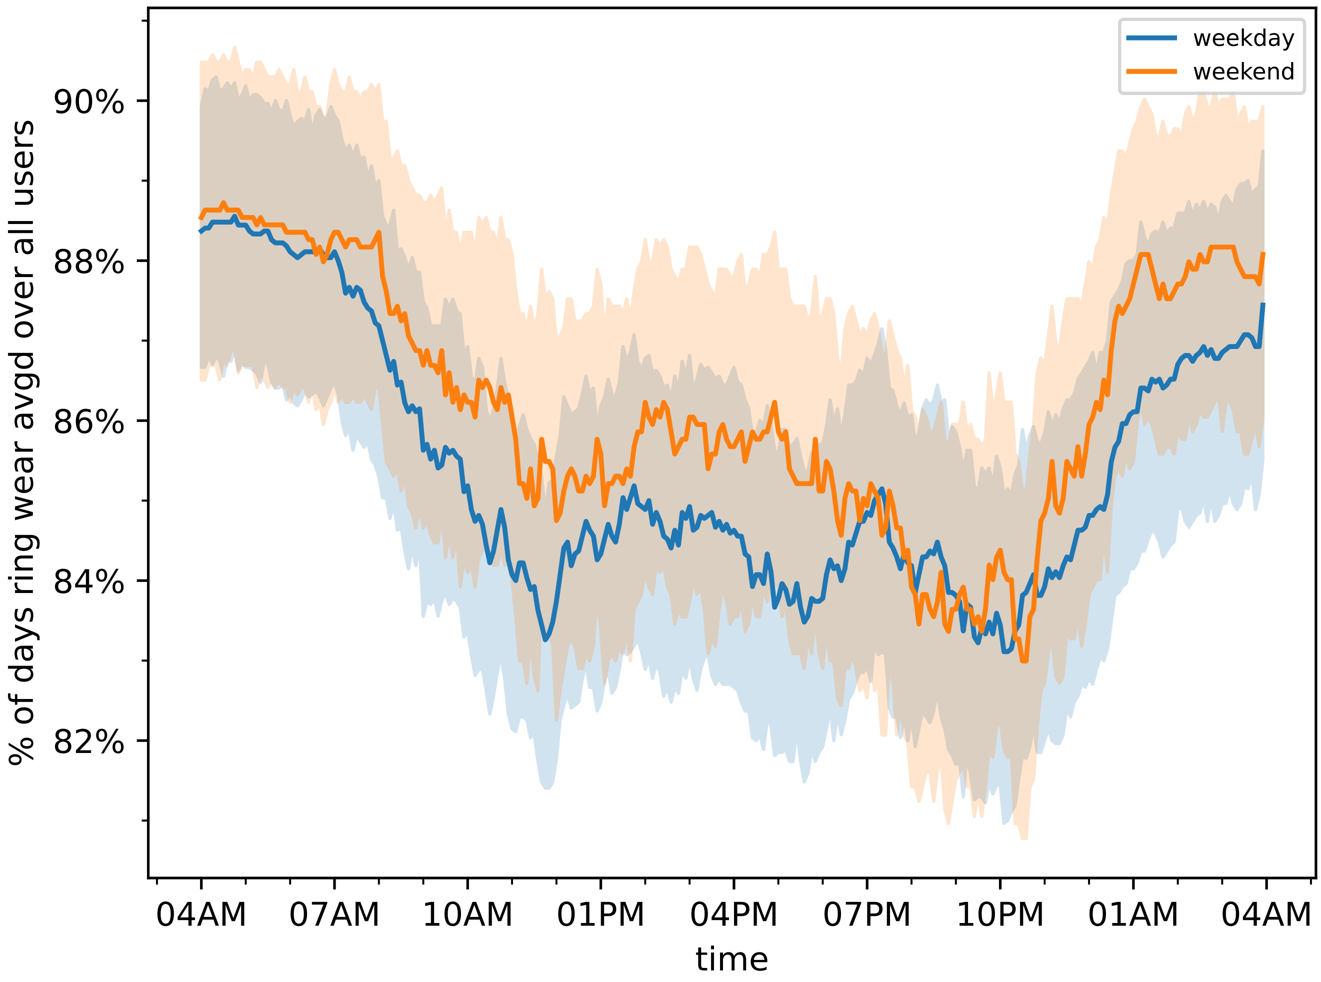


Figure S3. **Ring wear compliance over the course of a day for Thanksgiving week.** For each user, we take the percentage of weekdays and weekends (excluding the week of Thanksgiving break) that they wear the ring at a given time. The solid curves show the average of this time series across all users, and the shaded areas indicate the 95% confidence interval. Dips in wear consistency are found in the morning and evening. Unlike during the weeks when school is in session, the dips in wear consistency for Thanksgiving week are consistent in timing for both weekdays and weekends.

## S-II. FIGURES: ACTIVITY TIME SERIES COMPARISON

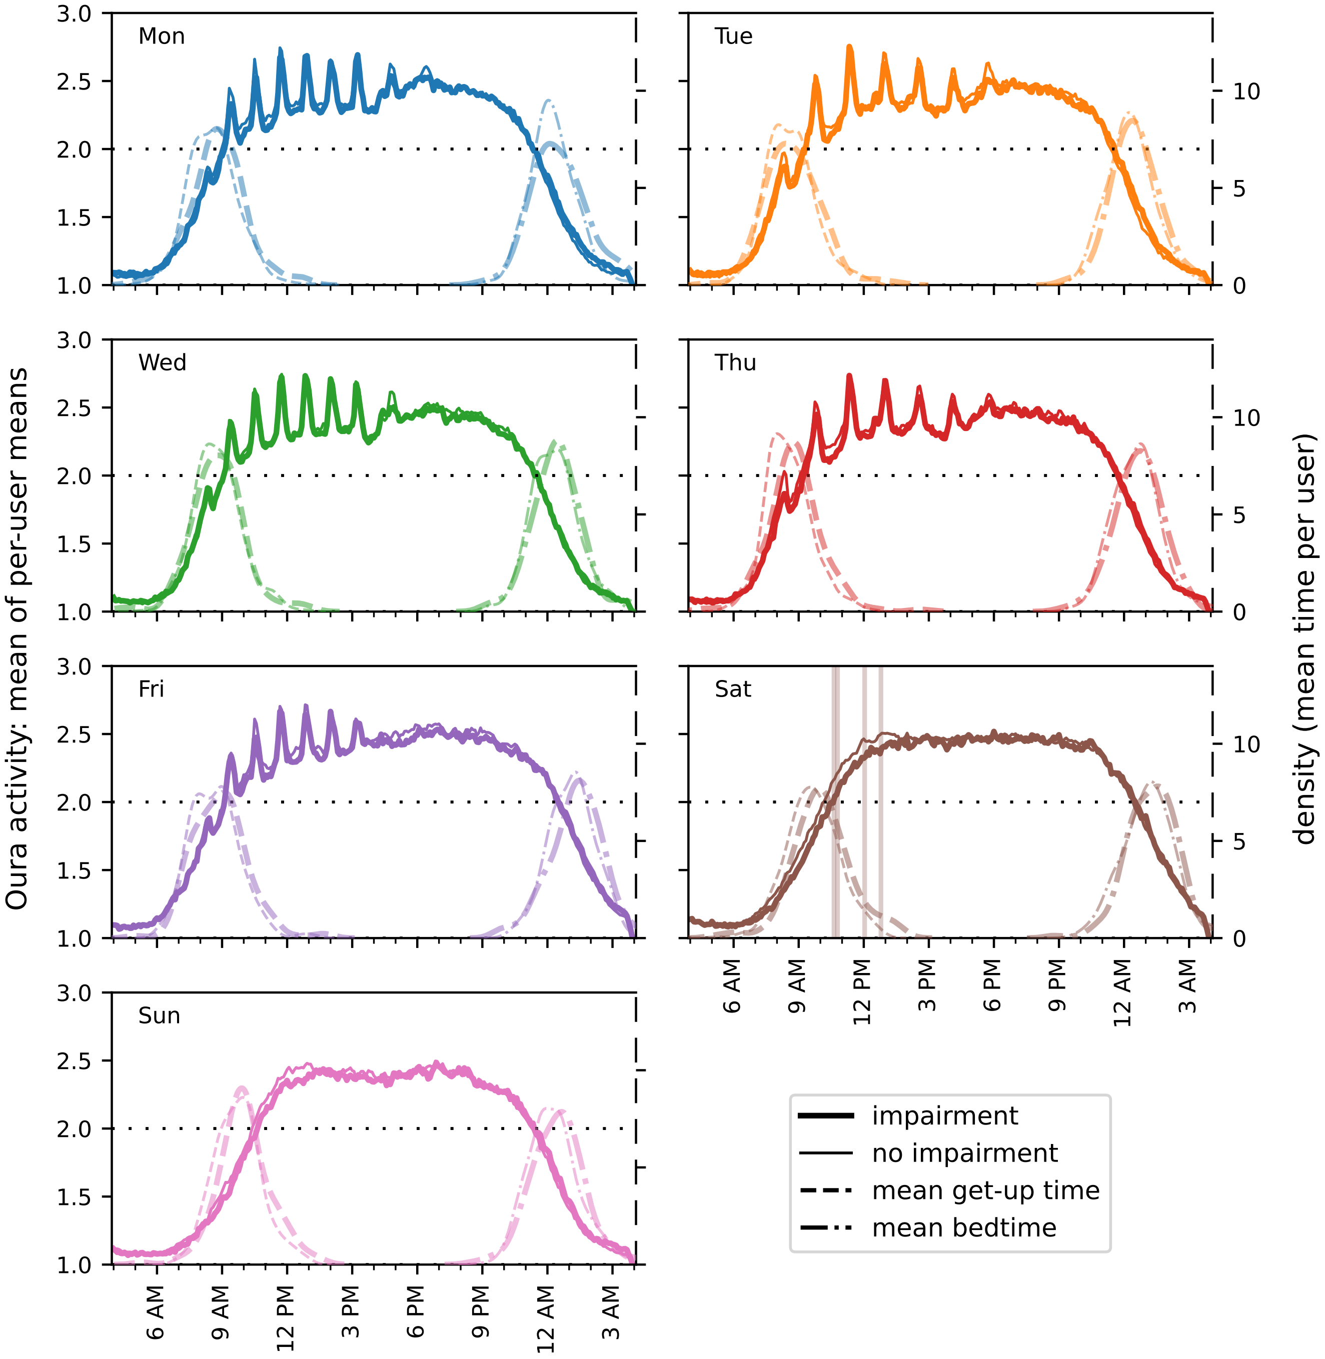


Figure S4. **Comparison of activity time series by impairment status.** Periods in the activity time series with differences statistically significant at $\alpha = 0.05$ according to statistical parametric mapping (SPM) are shaded.

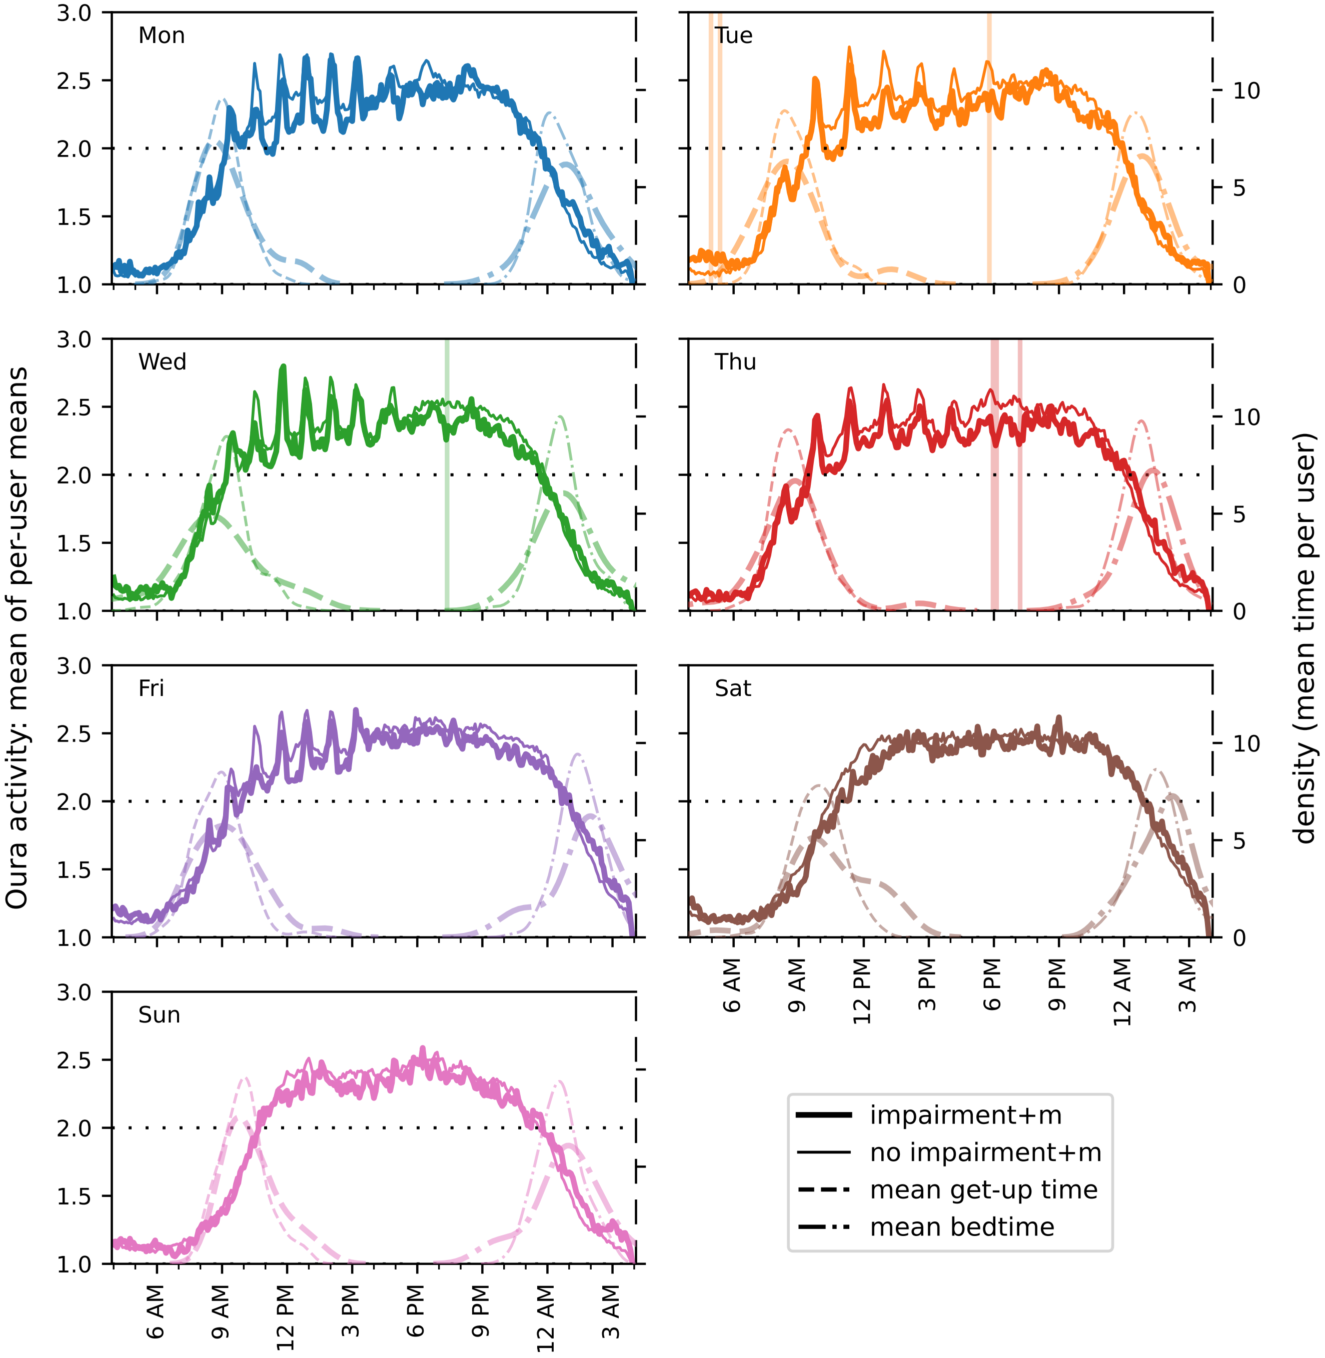


Figure S5. **Comparison of activity time series by impairment status for males.** Periods in the activity time series with differences statistically significant at $\alpha = 0.05$ according to statistical parametric mapping (SPM) are shaded.

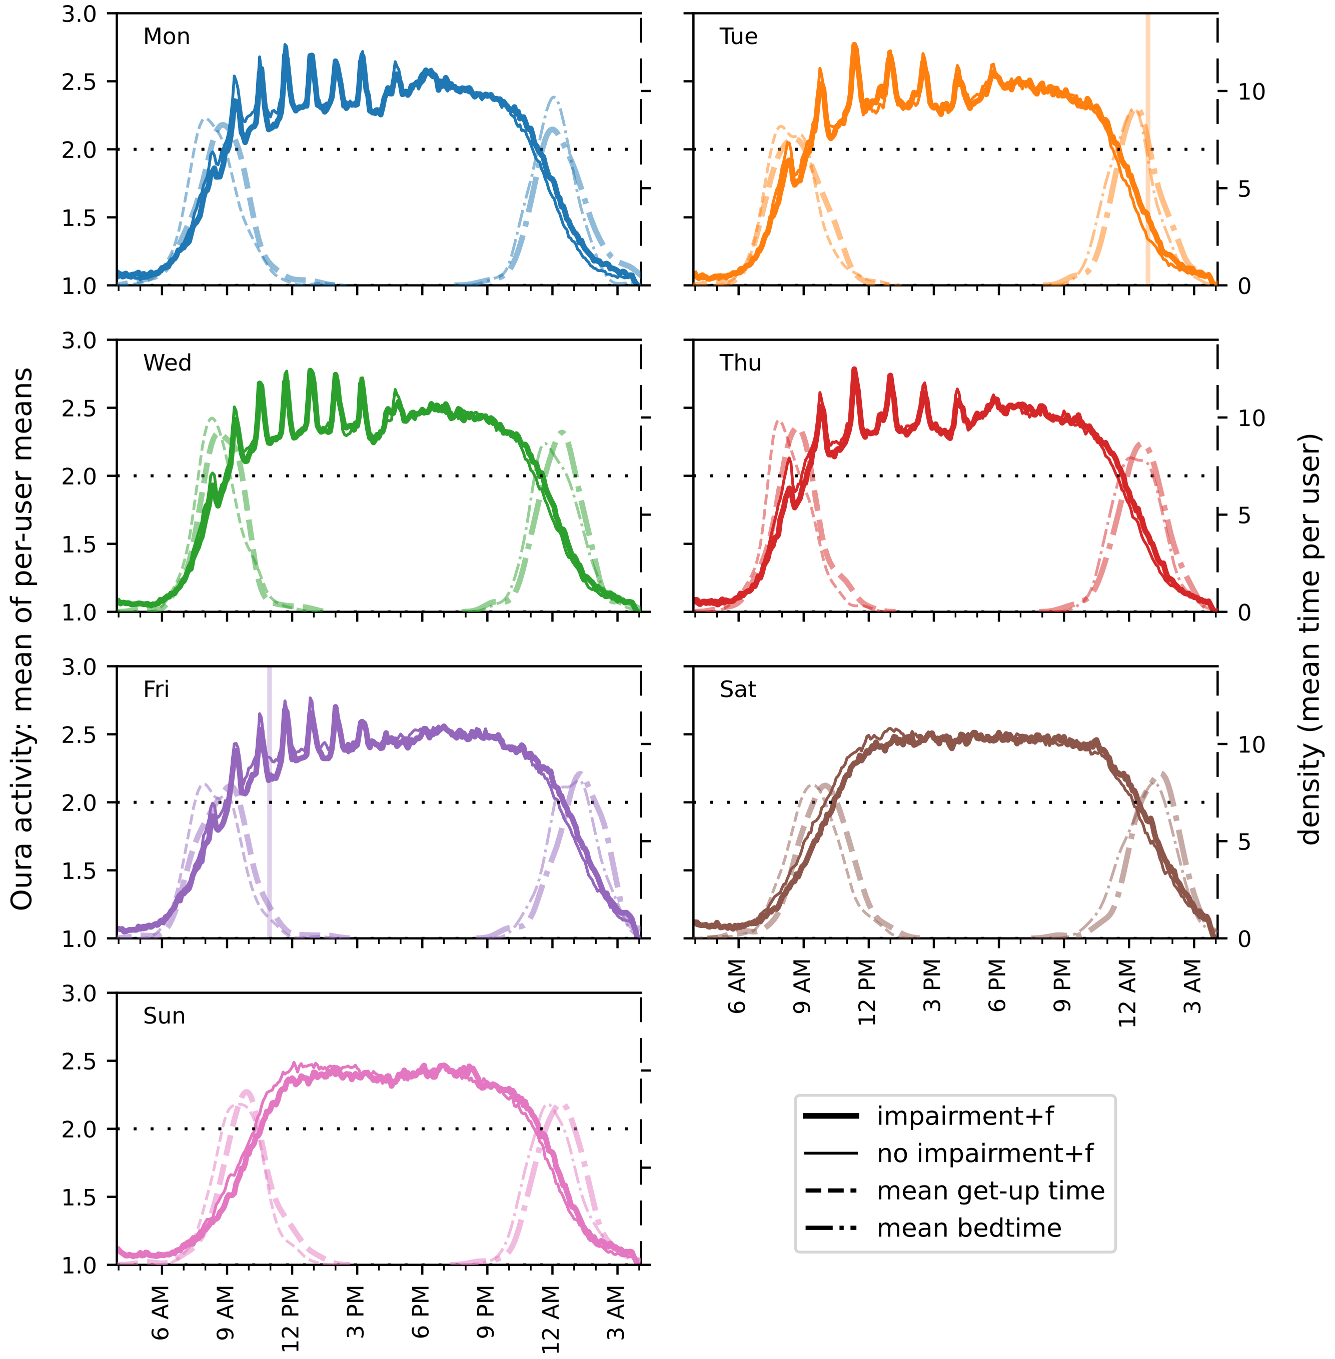


Figure S6. **Comparison of activity time series by impairment status for females.** Periods in the activity time series with differences statistically significant at $\alpha = 0.05$ according to statistical parametric mapping (SPM) are shaded.

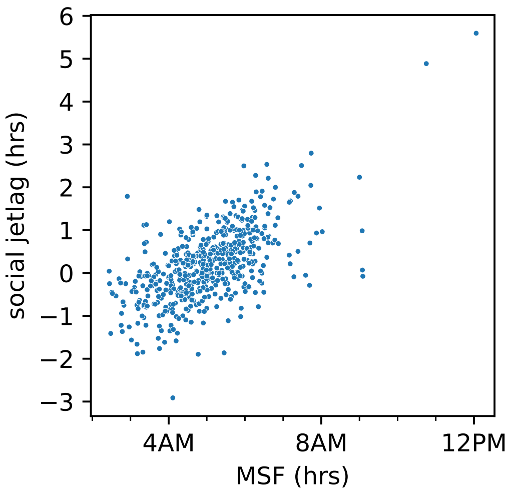


Figure S7. **Jetlag vs. sleep period midpoint during free days (MSF).** Social jetlag is higher for late-night chronotypes, which is characterized by a late mean sleep period midpoint calculated from Thanksgiving break.

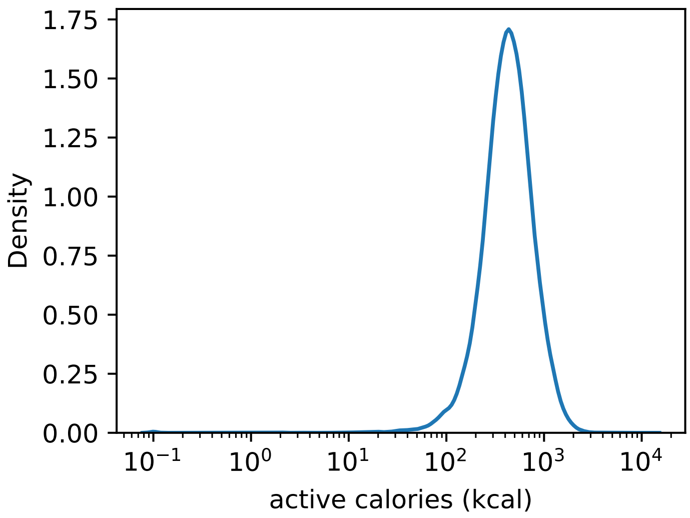


Figure S8. **Histogram of active calories.** Zero calorie counts form a very small minority and were assigned a value of 0.1 to calculate the log transform.

Table S1. **Count by gender and mental health impairment.** A count breakdown by gender and reported impairment due to anxiety or depression of the $N = 572$ individuals who had at least three (3) weeks of activity data for a particular day of the week is given in the table below.

| | *Female* | | *Male* | | *Non-binary* | |
|---|---|---|---|---|---|---|
| | *No impairment* | *Impairment* | *No impairment* | *Impairment* | *No impairment* | *Impairment* |
| Monday | 228 | 140 | 131 | 28 | 12 | 22 |
| Tuesday | 228 | 139 | 131 | 28 | 12 | 22 |
| Wednesday | 227 | 142 | 132 | 29 | 12 | 22 |
| Thursday | 227 | 140 | 129 | 29 | 12 | 22 |
| Friday | 227 | 141 | 130 | 28 | 12 | 23 |
| Saturday | 229 | 143 | 131 | 28 | 12 | 22 |
| Sunday | 228 | 140 | 131 | 28 | 12 | 22 |

## S-III. TABLES

Table S2. **Mixed-effects Gaussian regression models predicting bedtimes for every sleep period using gender.** The participant ID, week number, and the day of the week as random effects. Thanksgiving week is excluded.

| *Response* | *Fixed Effect* | *Coeff* | *2.5 CI* | *97.5 CI* | *p-value* |
|---|---|---|---|---|---|
| bedtime start (hrs from 12mn) | Gender - m (0=f) | 0.553 | 0.361 | 0.744 | **<0.001** |
| | Gender - nb (0=f) | 0.241 | -0.118 | 0.600 | 0.189 |
| | Gender (0=f, 1 otherwise) | 0.497 | 0.318 | 0.676 | **<0.001** |
| | Gender (0=m, 1 otherwise) | -0.532 | -0.721 | -0.343 | **<0.001** |
| | Gender (0=nb, 1 otherwise) | -0.074 | -0.438 | 0.290 | 0.690 |
| bedtime end (hrs from 12mn) | Gender - m (0=f) | 0.349 | 0.174 | 0.524 | **<0.001** |
| | Gender - nb (0=f) | 0.357 | 0.028 | 0.685 | **0.034** |
| | Gender (0=f, 1 otherwise) | 0.350 | 0.187 | 0.514 | **<0.001** |
| | Gender (0=m, 1 otherwise) | -0.318 | -0.492 | -0.145 | **<0.001** |
| | Gender (0=nb, 1 otherwise) | -0.251 | -0.579 | 0.077 | 0.134 |
| bedtime duration (hrs) | Gender - m (0=f) | -0.132 | -0.259 | -0.005 | **0.042** |
| | Gender - nb (0=f) | 0.112 | -0.126 | 0.350 | 0.358 |
| | Gender (0=f, 1 otherwise) | -0.088 | -0.208 | 0.031 | 0.146 |
| | Gender (0=m, 1 otherwise) | 0.142 | 0.016 | 0.267 | **0.027** |
| | Gender (0=nb, 1 otherwise) | -0.151 | -0.387 | 0.084 | 0.208 |
| sleep efficiency (%) | Gender - m (0=f) | -4.072 | -4.683 | -3.461 | **<0.001** |
| | Gender - nb (0=f) | -1.480 | -2.627 | -0.334 | **0.012** |
| | Gender (0=f, 1 otherwise) | -3.610 | -4.191 | -3.030 | **<0.001** |
| | Gender (0=m, 1 otherwise) | 3.945 | 3.339 | 4.551 | **<0.001** |
| | Gender (0=nb, 1 otherwise) | 0.255 | -1.036 | 1.545 | 0.699 |
